# Supplementary material for: A Lightweight Modular Continuum Manipulator with IMU-based Force Estimation
Source: arXiv:2211.11874 source file (2022-11-21)
Supplement: Supplementary file 1 [file appendix.tex]

%%%%%%%%%%%%%%%%%%%%%%%%%%%%%%%%%%%%%%%%%%%%%%%%%%%%%%%%%%%%%%%%%%%%%%
\appendix       %%% starting appendix
\section*{Appendix A: Derivation of $ \mb{J}_{\omega\psi}$}\label{app:J_omega_psi}
We express the rotation matrix $ \mb{R} $ in (\ref{eqn:diff_R_paul}) with the three unit vectors for derivation convenience:
\begin{equation}
	\mb{R} \triangleq
	\left[
	\begin{array}{c;{2pt/2pt}c;{2pt/2pt}c}
			\uvec{n}_x & \uvec{n}_y & \uvec{n}_z	
	\end{array}
	\right] 
\end{equation}
It allows us to rewrite (\ref{eqn:diff_R_paul}) as:
\begin{equation}
\begin{array}{rl}
	% line 1
	\rm{d}\; \mb{R} = &
	\left[(\bs{\omega}\;\rm{d}t)^\wedge\right]\; \mb{R} = 
	\left[
	\begin{array}{c;{2pt/2pt}c;{2pt/2pt}c}
	\left[(\bs{\omega})^\wedge\right] \uvec{n}_x \phantom{\;} & \phantom{\;}
	\left[(\bs{\omega})^\wedge\right] \uvec{n}_y \phantom{\;} & \phantom{\;}
	\left[(\bs{\omega})^\wedge\right] \uvec{n}_z	\phantom{\;}
	\end{array}	
	\right] \;\rm{d}t \\	
	% line 2
	= & 
	\left[
	\begin{array}{c;{2pt/2pt}c;{2pt/2pt}c}
	\left[(\uvec{n}_x)^\wedge\right]\T  \bs{\omega} \phantom{\;}& \phantom{\;} 
	\left[(\uvec{n}_y)^\wedge\right]\T  \bs{\omega} \phantom{\;} & \phantom{\;} 
	\left[(\uvec{n}_z)^\wedge\right]\T  \bs{\omega} \phantom{\;}
	\end{array}	
	\right] \;\rm{d}t
\end{array}
\label{eqn:diff_R_paul_1}
\end{equation}\par
Let us use $ \vect{\cdot}$ to denote the vectorization of a matrix by stacking the columns of the matrix on top one another. We then can vectorize (\ref{eqn:diff_R_paul_1}) as:
\begin{align}
	&
	\vect{\rm{d}\; \mb{R}} = 
	\left[
	\begin{array}{c}
	\left[(\uvec{n}_x)^\wedge\right]\T  \bs{\omega} \phantom{\Bigg|}\\\hdashline
	\left[(\uvec{n}_y)^\wedge\right]\T  \bs{\omega} \phantom{\Bigg|}\\\hdashline
	\left[(\uvec{n}_z)^\wedge\right]\T  \bs{\omega} \phantom{\Bigg|}
	\end{array}
	\right] \;\rm{d}t=
\underbrace{		\left[
	\begin{array}{c}
	\left[(\uvec{n}_x)^\wedge\right]\T   \phantom{\Bigg|}\\\hdashline
	\left[(\uvec{n}_y)^\wedge\right]\T  \phantom{\Bigg|}\\\hdashline
	\left[(\uvec{n}_z)^\wedge\right]\T  \phantom{\Bigg|}
	\end{array} 
	\right]}_{\triangleq \;\mb{D}} \; \bs{\omega} \;\rm{d}t\\
	\text{Or,}\quad &
	\vect{\rm{d}\; \mb{R}} = \mb{D}\;\bs{\omega} \;\rm{d}t, \quad \mb{D}\in\realfield{9\times 3}
	\label{eqn:diff_R_paul_2}
\end{align}\par
Thereby, we have achieved the vectorization and rearrangement of (\ref{eqn:diff_R_paul}), arriving at (\ref{eqn:diff_R_paul_2}). In addition, we note that matrix $ \mb{D} $ has linearly independent columns and has a rank of 3, which suggests that it has a particular pseudoinverse as a \textit{left inverse}.\par
Next, we consider the vectorization of (\ref{eqn:diff_R_full}):
\begin{align}
	% line 1
	& 
	\begin{array}{rl}
	\vect{\rm{d}\; \mb{R}} = &
	\left[\vect{\tfrac{\partial \mb{R}}{\partial \theta}}\right] \; \dot{\theta}\;\rm{d}t + 
	\left[\vect{\tfrac{\partial \mb{R}}{\partial \phi}}\right] \; \dot{\phi}\;\rm{d}t \\[12pt]
	=& 
	\underbrace{
	\left[\begin{array}{c;{2pt/2pt}c}
		\phantom{\;}\vect{\tfrac{\partial \mb{R}}{\partial \theta}} \phantom{\;\Bigg|}& 
		\phantom{\;}\vect{\tfrac{\partial \mb{R}}{\partial \phi}}\phantom{\;\Bigg|}
	\end{array}
	\right]}_{\triangleq\;\mb{E}} 
	\underbrace{\begin{bmatrix}
		\dot{\theta}\\\dot{\phi}
	\end{bmatrix}}_{\dot{\bs{\psi}}}
	\end{array} \;\rm{d}t\\
	% line 2
	\text{Or,}\quad & \vect{\rm{d}\; \mb{R}} = \mb{E}\;\dot{\bs{\psi}}\;\rm{d}t, \quad \mb{E}\in\realfield{9\times 2}
	\label{eqn:diff_R_full_1}
\end{align}
where the two derivative matrices, $ \tfrac{\partial \mb{R}}{\partial \theta} $ and $ \tfrac{\partial \mb{R}}{\partial \phi} $, can be computed easily by recalling that $ \mb{R} $ represents the orientation of the last link ($ \mb{R} = \mb{R}_{N_l} $) and by using the iterative computation methods shown in (\ref{eqn:d_Ri_d_theta}) and (\ref{eqn:d_Ri_d_phi}). Thereby, we have achieved the vectorization and rearrangement of (\ref{eqn:diff_R_full}), arriving at (\ref{eqn:diff_R_full_1}).\par
Finally, by equating the right-hand sides of (\ref{eqn:diff_R_paul_2}) and (\ref{eqn:diff_R_full_1}), we obtain the expression of the Jacobian matrix:
\begin{equation}
	\bs{\omega} = 
	\underbrace{\left(\phantom{\big|}\mb{D}^+\;\mb{E}\phantom{\big|}\right)}_{\triangleq \;\mb{J}_{\omega\psi}} \; \dot{\bs{\psi}}
\end{equation}
where $ (\cdot)^+ $ denotes the pseudoinverse matrix operation, which, in this case, is computed as:
\begin{equation}
	\mb{D}^+ = \left(\mb{D}\T\;\mb{D}\right)^{-1}\;\mb{D}\T
\end{equation}
%Avoid Appendices if possible.
